# Supplementary material for: Simulating Charged Defects at Database Scale
Source: arXiv:2403.05689 source file (2024-03-08)
Supplement: Supplementary file 1 [file supp_no_blank.pdf]

# Supplemental Materials for "Simulating Charged Defects at Database Scale"

(Dated: February 7, 2024)

The exact values of the transition levels for all of the native defects in GaN, $Ga_2O_3$ and $STiO_3$ from Figures (4-6) of the manuscript are tabulated in Tables (I–III) below. For each charge state transition level, we reported the formation energy for two distinct chemical potential conditions. The two charge states involved in each transition is reported. We also report the formation energies at the VBM or CBM, we only involves a single charge state.

TABLE I: **GaN: PBE-Sol**: The transitions levels of native defects in GaN under Ga-rich and N-rich conditions. calculated using the PBE-Sol functional. This data corresponds to Figure 4(c) of the manuscript.

| Defect Name | Transition | $E_{\text{Fermi}}$ | $E_{\text{form}}$ (Ga-rich) | $E_{\text{form}}$ (N-rich) |
|---|---|---|---|---|
| $Ga_N$ | VBM $\rightarrow$ 3 | 0.00 | 3.82 | 6.45 |
| | 3 $\rightarrow$ 2 | 0.21 | 4.46 | 7.09 |
| | 2 $\rightarrow$ 1 | 0.65 | 5.34 | 7.97 |
| | 1 $\rightarrow$ 0 | 1.45 | 6.14 | 8.76 |
| | 0 $\rightarrow$ CBM | 1.92 | 6.14 | 8.76 |
| $Ga_{i,I}$ | VBM $\rightarrow$ 3 | 0.00 | 3.21 | 4.52 |
| | 3 $\rightarrow$ 2 | 1.20 | 6.80 | 8.12 |
| | 2 $\rightarrow$ 1 | 1.53 | 7.46 | 8.77 |
| | 1 $\rightarrow$ CBM | 1.92 | 7.85 | 9.16 |
| $Ga_{i,II}$ | VBM $\rightarrow$ 3 | 0.00 | 4.23 | 5.54 |
| | 3 $\rightarrow$ 2 | 1.26 | 8.02 | 9.34 |
| | 2 $\rightarrow$ CBM | 1.92 | 9.33 | 10.64 |

Continued on next page

TABLE I: **GaN: PBE-Sol**: The transitions levels of native defects in GaN under Ga-rich and N-rich conditions. calculated using the PBE-Sol functional. This data corresponds to Figure 4(c) of the manuscript. (Continued)

| Defect Name | Transition | $E_{\text{Fermi}}$ | $E_{\text{form}}$ (Ga-rich) | $E_{\text{form}}$ (N-rich) |
|---|---|---|---|---|
| $N_{Ga}$ | VBM $\rightarrow$ 1 | 0.00 | 8.97 | 6.34 |
| | 1 $\rightarrow$ 0 | 0.69 | 9.66 | 7.03 |
| | 0 $\rightarrow$ $-1$ | 1.88 | 9.66 | 7.03 |
| | $-1$ $\rightarrow$ CBM | 1.92 | 9.62 | 7.00 |
| $N_{i,I}$ | VBM $\rightarrow$ 1 | 0.00 | 5.46 | 4.15 |
| | 1 $\rightarrow$ CBM | 1.92 | 7.37 | 6.06 |
| $N_{i,II}$ | VBM $\rightarrow$ 2 | 0.00 | 4.93 | 3.61 |
| | 2 $\rightarrow$ 1 | 0.49 | 5.90 | 4.59 |
| | 1 $\rightarrow$ 0 | 0.61 | 6.03 | 4.71 |
| | 0 $\rightarrow$ $-1$ | 1.83 | 6.03 | 4.71 |
| | $-1$ $\rightarrow$ CBM | 1.92 | 5.94 | 4.62 |
| $v_{Ga}$ | VBM $\rightarrow$ 0 | 0.00 | 7.81 | 6.50 |
| | 0 $\rightarrow$ $-1$ | 0.64 | 7.81 | 6.50 |
| | $-1$ $\rightarrow$ $-2$ | 1.22 | 7.23 | 5.92 |
| | $-2$ $\rightarrow$ $-3$ | 1.81 | 6.05 | 4.74 |
| | $-3$ $\rightarrow$ CBM | 1.92 | 5.74 | 4.43 |
| $v_N$ | VBM $\rightarrow$ 1 | 0.00 | 0.79 | 2.11 |
| | 1 $\rightarrow$ CBM | 1.92 | 2.71 | 4.02 |

TABLE II: **GaN: HSE06**: The transitions levels of native defects in GaN under Ga-rich and N-rich conditions, calculated using the HSE06 functional. This data corresponds to Figure 4(b) of the manuscript.

| Defect Name | Transition | $E_{\text{Fermi}}$ | $E_{\text{form}}$ (Ga-rich) | $E_{\text{form}}$ (N-rich) |
|---|---|---|---|---|
| $Ga_N$ | VBM $\rightarrow$ 4 | 0.00 | 2.96 | 5.59 |
| | $4 \rightarrow 3$ | 0.03 | 3.10 | 5.73 |
| | $3 \rightarrow 2$ | 0.67 | 5.00 | 7.63 |
| | $2 \rightarrow 1$ | 0.89 | 5.44 | 8.07 |
| | $1 \rightarrow 0$ | 2.11 | 6.66 | 9.29 |
| | $0 \rightarrow -1$ | 2.75 | 6.66 | 9.29 |
| | $-1 \rightarrow$ CBM | 3.26 | 6.16 | 8.79 |
| $Ga_{i,I}$ | VBM $\rightarrow$ 3 | 0.00 | 1.71 | 3.02 |
| | $3 \rightarrow 2$ | 1.79 | 7.09 | 8.40 |
| | $2 \rightarrow 1$ | 2.33 | 8.17 | 9.48 |
| | $1 \rightarrow$ CBM | 3.26 | 9.09 | 10.41 |
| $Ga_{i,II}$ | VBM $\rightarrow$ 3 | 0.00 | 2.51 | 3.82 |
| | $3 \rightarrow 2$ | 2.60 | 10.31 | 11.63 |
| | $2 \rightarrow 1$ | 2.88 | 10.87 | 12.18 |
| | $1 \rightarrow$ CBM | 3.26 | 11.25 | 12.56 |
| $N_{Ga}$ | VBM $\rightarrow$ 1 | 0.00 | 9.45 | 6.82 |
| | $1 \rightarrow -1$ | 1.47 | 10.92 | 8.29 |
| | $-1 \rightarrow$ CBM | 3.26 | 9.14 | 6.51 |

Continued on next page

TABLE II: **GaN: HSE06**: The transitions levels of native defects in GaN under Ga-rich and N-rich conditions, calculated using the HSE06 functional. This data corresponds to Figure 4(b) of the manuscript. (Continued)

| Defect Name | Transition | $E_{\mathrm{Fermi}}$ | $E_{\mathrm{form}}$ (Ga-rich) | $E_{\mathrm{form}}$ (N-rich) |
|---|---|---|---|---|
| $N_{i,I}$ | VBM $\rightarrow$ 2 | 0.00 | 7.70 | 6.38 |
| | $2 \rightarrow 1$ | 0.22 | 8.14 | 6.83 |
| | $1 \rightarrow 0$ | 1.50 | 9.42 | 8.11 |
| | $0 \rightarrow -1$ | 2.37 | 9.42 | 8.11 |
| | $-1 \rightarrow$ CBM | 3.26 | 8.54 | 7.22 |
| $N_{i,II}$ | VBM $\rightarrow$ 2 | 0.00 | 4.06 | 2.75 |
| | $2 \rightarrow 1$ | 0.75 | 5.57 | 4.25 |
| | $1 \rightarrow 0$ | 1.43 | 6.25 | 4.93 |
| | $0 \rightarrow -1$ | 2.94 | 6.25 | 4.93 |
| | $-1 \rightarrow$ CBM | 3.26 | 5.93 | 4.61 |
| $v_{Ga}$ | VBM $\rightarrow$ 1 | 0.00 | 7.22 | 5.90 |
| | $1 \rightarrow 0$ | 0.60 | 7.82 | 6.51 |
| | $0 \rightarrow -1$ | 1.49 | 7.82 | 6.51 |
| | $-1 \rightarrow -2$ | 1.96 | 7.35 | 6.04 |
| | $-2 \rightarrow -3$ | 2.52 | 6.24 | 4.93 |
| | $-3 \rightarrow$ CBM | 3.26 | 4.02 | 2.71 |
| $v_N$ | VBM $\rightarrow$ 3 | 0.00 | -0.41 | 0.90 |
| | $3 \rightarrow 2$ | 0.08 | -0.17 | 1.14 |
| | $2 \rightarrow 1$ | 0.20 | 0.08 | 1.39 |
| | $1 \rightarrow 0$ | 3.14 | 3.01 | 4.32 |
| | $0 \rightarrow$ CBM | 3.26 | 3.01 | 4.32 |

TABLE III: **$Ga_2O_3$: PBE-Sol**: The transitions levels of native defects in $Ga_2O_3$ under Ga-rich and N-rich conditions, calculated using the PBE-Sol functional. This data corresponds to Figure 5(a) of the manuscript.

| Defect Name | Transition | $E_{\mathrm{Fermi}}$ | $E_{\mathrm{form}}$ (Ga-rich) | $E_{\mathrm{form}}$ (N-rich) |
|---|---|---|---|---|
| $Ga_{O,I}$ | VBM $\rightarrow$ 3 | 0.00 | -1.65 | 7.81 |
| | 3 $\rightarrow$ 2 | 1.61 | 3.19 | 12.64 |
| | 2 $\rightarrow$ 1 | 2.01 | 3.98 | 13.44 |
| | 1 $\rightarrow$ CBM | 2.26 | 4.23 | 13.69 |
| $Ga_{O,II}$ | VBM $\rightarrow$ 3 | 0.00 | -0.56 | 8.89 |
| | 3 $\rightarrow$ 2 | 1.20 | 3.04 | 12.49 |
| | 2 $\rightarrow$ 1 | 1.57 | 3.77 | 13.23 |
| | 1 $\rightarrow$ CBM | 2.26 | 4.46 | 13.92 |
| $Ga_{O,III}$ | VBM $\rightarrow$ 3 | 0.00 | -0.30 | 9.16 |
| | 3 $\rightarrow$ 1 | 1.49 | 4.18 | 13.64 |
| | 1 $\rightarrow$ CBM | 2.26 | 4.95 | 14.41 |
| $Ga_{i,I}$ | VBM $\rightarrow$ 3 | 0.00 | -0.66 | 5.01 |
| | 3 $\rightarrow$ 2 | 1.54 | 3.96 | 9.64 |
| | 2 $\rightarrow$ 1 | 1.74 | 4.37 | 10.04 |
| | 1 $\rightarrow$ CBM | 2.26 | 4.89 | 10.56 |
| $Ga_{i,II}$ | VBM $\rightarrow$ 3 | 0.00 | -0.98 | 4.70 |
| | 3 $\rightarrow$ 2 | 2.17 | 5.54 | 11.21 |
| | 2 $\rightarrow$ CBM | 2.26 | 5.72 | 11.39 |
| $O_{Ga,I}$ | VBM $\rightarrow$ 1 | 0.00 | 12.61 | 3.15 |
| | 1 $\rightarrow$ 0 | 0.23 | 12.84 | 3.38 |
| | 0 $\rightarrow$ $-1$ | 1.44 | 12.84 | 3.38 |
| | $-1$ $\rightarrow$ CBM | 2.26 | 12.02 | 2.56 |

Continued on next page

TABLE III: **$Ga_2O_3$: PBE-Sol**: The transitions levels of native defects in $Ga_2O_3$ under Ga-rich and N-rich conditions, calculated using the PBE-Sol functional. This data corresponds to Figure 5(a) of the manuscript. (Continued)

| Defect Name | Transition | $E_{Fermi}$ | $E_{form}$ (Ga-rich) | $E_{form}$ (N-rich) |
|---|---|---|---|---|
| $O_{Ga,II}$ | VBM $\rightarrow$ 0 | 0.00 | 13.67 | 4.21 |
| | 0 $\rightarrow$ $-2$ | 1.81 | 13.67 | 4.21 |
| | $-2$ $\rightarrow$ CBM | 2.26 | 12.78 | 3.32 |
| $O_{i,I}$ | VBM $\rightarrow$ 1 | 0.00 | 8.69 | 4.90 |
| | 1 $\rightarrow$ 0 | 0.26 | 8.95 | 5.16 |
| | 0 $\rightarrow$ $-1$ | 1.48 | 8.95 | 5.16 |
| | $-1$ $\rightarrow$ CBM | 2.26 | 8.16 | 4.38 |
| $O_{i,II}$ | VBM $\rightarrow$ 1 | 0.00 | 6.19 | 2.41 |
| | 1 $\rightarrow$ 0 | 0.63 | 6.83 | 3.04 |
| | 0 $\rightarrow$ $-1$ | 2.25 | 6.83 | 3.04 |
| | $-1$ $\rightarrow$ CBM | 2.26 | 6.82 | 3.04 |
| $v_{Ga,I}$ | VBM $\rightarrow$ 0 | 0.00 | 10.42 | 4.74 |
| | 0 $\rightarrow$ $-1$ | 0.37 | 10.42 | 4.74 |
| | $-1$ $\rightarrow$ $-2$ | 0.95 | 9.83 | 4.16 |
| | $-2$ $\rightarrow$ $-3$ | 1.74 | 8.26 | 2.59 |
| | $-3$ $\rightarrow$ CBM | 2.26 | 6.69 | 1.01 |
| $v_{Ga,II}$ | VBM $\rightarrow$ 0 | 0.00 | 10.12 | 4.45 |
| | 0 $\rightarrow$ $-1$ | 0.53 | 10.12 | 4.45 |
| | $-1$ $\rightarrow$ $-2$ | 1.12 | 9.54 | 3.86 |
| | $-2$ $\rightarrow$ $-3$ | 1.87 | 8.04 | 2.36 |
| | $-3$ $\rightarrow$ CBM | 2.26 | 6.86 | 1.19 |

Continued on next page

TABLE III: **$Ga_2O_3$: PBE-Sol**: The transitions levels of native defects in $Ga_2O_3$ under Ga-rich and N-rich conditions, calculated using the PBE-Sol functional. This data corresponds to Figure 5(a) of the manuscript. (Continued)

| Defect Name | Transition | $E_{\text{Fermi}}$ | $E_{\text{form}}$ (Ga-rich) | $E_{\text{form}}$ (N-rich) |
|---|---|---|---|---|
| $v_{O,I}$ | VBM $\rightarrow$ 2 | 0.00 | -0.81 | 2.98 |
| | 2 $\rightarrow$ 0 | 0.82 | 0.83 | 4.61 |
| | 0 $\rightarrow$ CBM | 2.26 | 0.83 | 4.61 |
| $v_{O,II}$ | VBM $\rightarrow$ 2 | 0.00 | -1.33 | 2.45 |
| | 2 $\rightarrow$ 0 | 1.40 | 1.46 | 5.25 |
| | 0 $\rightarrow$ CBM | 2.26 | 1.46 | 5.25 |
| $v_{O,III}$ | VBM $\rightarrow$ 2 | 0.00 | -1.54 | 2.24 |
| | 2 $\rightarrow$ 0 | 1.38 | 1.22 | 5.00 |
| | 0 $\rightarrow$ CBM | 2.26 | 1.22 | 5.00 |

TABLE IV: **$Ga_2O_3$: HSE06**: The transitions levels of native defects in $Ga_2O_3$ under Ga-rich and N-rich conditions, calculated using the HSE06 functional. This data corresponds to Figure 5(b) of the manuscript.

| Defect Name | Transition | $E_{\text{Fermi}}$ | $E_{\text{form}}$ (Ga-rich) | $E_{\text{form}}$ (N-rich) |
|---|---|---|---|---|
| $Ga_{O,I}$ | VBM $\rightarrow$ 3 | 0.00 | -3.24 | 6.21 |
| | 3 $\rightarrow$ 2 | 1.56 | 1.45 | 10.91 |
| | 2 $\rightarrow$ 1 | 3.35 | 5.02 | 14.48 |
| | 1 $\rightarrow$ CBM | 4.21 | 5.88 | 15.34 |

Continued on next page

TABLE IV: **$Ga_2O_3$: HSE06**: The transitions levels of native defects in $Ga_2O_3$ under Ga-rich and N-rich conditions, calculated using the HSE06 functional. This data corresponds to Figure 5(b) of the manuscript. (Continued)

| Defect Name | Transition | $E_{Fermi}$ | $E_{form}$ (Ga-rich) | $E_{form}$ (N-rich) |
|---|---|---|---|---|
| $Ga_{O,II}$ | VBM $\rightarrow$ 4 | 0.00 | -5.20 | 4.26 |
| | 4 $\rightarrow$ 3 | 0.09 | -4.84 | 4.62 |
| | 3 $\rightarrow$ 2 | 2.84 | 3.42 | 12.87 |
| | 2 $\rightarrow$ 1 | 3.31 | 4.35 | 13.81 |
| | 1 $\rightarrow$ 0 | 4.17 | 5.21 | 14.67 |
| | 0 $\rightarrow$ CBM | 4.21 | 5.21 | 14.67 |
| $Ga_{O,III}$ | VBM $\rightarrow$ 3 | 0.00 | -3.62 | 5.83 |
| | 3 $\rightarrow$ 2 | 2.10 | 2.68 | 12.14 |
| | 2 $\rightarrow$ 1 | 2.83 | 4.14 | 13.60 |
| | 1 $\rightarrow$ 0 | 3.63 | 4.94 | 14.40 |
| | 0 $\rightarrow$ CBM | 4.21 | 4.94 | 14.40 |
| $Ga_{i,I}$ | VBM $\rightarrow$ 3 | 0.00 | -4.52 | 1.15 |
| | 3 $\rightarrow$ 1 | 3.15 | 4.94 | 10.62 |
| | 1 $\rightarrow$ CBM | 4.21 | 5.99 | 11.67 |
| $Ga_{i,II}$ | VBM $\rightarrow$ 3 | 0.00 | -4.53 | 1.14 |
| | 3 $\rightarrow$ 2 | 3.88 | 7.10 | 12.78 |
| | 2 $\rightarrow$ 0 | 3.93 | 7.20 | 12.87 |
| | 0 $\rightarrow$ CBM | 4.21 | 7.20 | 12.87 |
| $O_{Ga,I}$ | VBM $\rightarrow$ 1 | 0.00 | 12.86 | 3.40 |
| | 1 $\rightarrow$ 0 | 0.79 | 13.65 | 4.19 |
| | 0 $\rightarrow$ $-1$ | 2.06 | 13.65 | 4.19 |
| | $-1$ $\rightarrow$ CBM | 4.21 | 11.50 | 2.04 |

Continued on next page

TABLE IV: **$Ga_2O_3$: HSE06**: The transitions levels of native defects in $Ga_2O_3$ under Ga-rich and N-rich conditions, calculated using the HSE06 functional. This data corresponds to Figure 5(b) of the manuscript. (Continued)

| Defect Name | Transition | $E_{\mathrm{Fermi}}$ | $E_{\mathrm{form}}$ (Ga-rich) | $E_{\mathrm{form}}$ (N-rich) |
|---|---|---|---|---|
| $O_{Ga,II}$ | VBM $\to$ 1 | 0.00 | 14.21 | 4.75 |
| | $1 \to -1$ | 0.95 | 15.16 | 5.70 |
| | $-1 \to -2$ | 3.85 | 12.26 | 2.80 |
| | $-2 \to$ CBM | 4.21 | 11.55 | 2.09 |
| $O_{i,I}$ | VBM $\to$ 1 | 0.00 | 8.44 | 4.66 |
| | $1 \to 0$ | 0.89 | 9.33 | 5.55 |
| | $0 \to -1$ | 2.34 | 9.33 | 5.55 |
| | $-1 \to -2$ | 4.08 | 7.59 | 3.81 |
| | $-2 \to$ CBM | 4.21 | 7.34 | 3.56 |
| $O_{i,II}$ | VBM $\to$ 1 | 0.00 | 5.18 | 1.39 |
| | $1 \to 0$ | 1.25 | 6.43 | 2.64 |
| | $0 \to -2$ | 3.68 | 6.43 | 2.64 |
| | $-2 \to$ CBM | 4.21 | 5.38 | 1.60 |
| $v_{Ga,I}$ | VBM $\to$ 1 | 0.00 | 9.88 | 4.21 |
| | $1 \to 0$ | 0.84 | 10.72 | 5.05 |
| | $0 \to -1$ | 1.29 | 10.72 | 5.05 |
| | $-1 \to -2$ | 2.08 | 9.93 | 4.25 |
| | $-2 \to -3$ | 2.77 | 8.55 | 2.87 |
| | $-3 \to$ CBM | 4.21 | 4.24 | -1.43 |

Continued on next page

TABLE IV: **$Ga_2O_3$: HSE06**: The transitions levels of native defects in $Ga_2O_3$ under Ga-rich and N-rich conditions, calculated using the HSE06 functional. This data corresponds to Figure 5(b) of the manuscript. (Continued)

| Defect Name | Transition | $E_{\text{Fermi}}$ | $E_{\text{form}}$ (Ga-rich) | $E_{\text{form}}$ (N-rich) |
|---|---|---|---|---|
| $v_{Ga,II}$ | VBM $\rightarrow$ 1 | 0.00 | 8.79 | 3.11 |
| | $1 \rightarrow 0$ | 1.16 | 9.95 | 4.27 |
| | $0 \rightarrow -1$ | 1.93 | 9.95 | 4.27 |
| | $-1 \rightarrow -2$ | 2.40 | 9.47 | 3.80 |
| | $-2 \rightarrow -3$ | 2.90 | 8.48 | 2.80 |
| | $-3 \rightarrow$ CBM | 4.21 | 4.55 | -1.12 |
| $v_{O,I}$ | VBM $\rightarrow$ 2 | 0.00 | -4.22 | -0.44 |
| | $2 \rightarrow 0$ | 2.62 | 1.02 | 4.81 |
| | $0 \rightarrow$ CBM | 4.21 | 1.02 | 4.81 |
| $v_{O,II}$ | VBM $\rightarrow$ 2 | 0.00 | -3.41 | 0.37 |
| | $2 \rightarrow 0$ | 2.00 | 0.59 | 4.37 |
| | $0 \rightarrow$ CBM | 4.21 | 0.59 | 4.37 |
| $v_{O,III}$ | VBM $\rightarrow$ 2 | 0.00 | -3.96 | -0.18 |
| | $2 \rightarrow 1$ | 2.59 | 1.22 | 5.00 |
| | $1 \rightarrow 0$ | 2.64 | 1.27 | 5.05 |
| | $0 \rightarrow$ CBM | 4.21 | 1.27 | 5.05 |

TABLE V: **$SrTiO_3$: HSE06**: The transitions levels of native defects in $SrTiO_3$ under Ti-rich and O-rich conditions, calculated using the HSE06 functional. This data corresponds to Figure 6 of the manuscript.

| Defect Name | Transition | $E_{Fermi}$ | $E_{form}$ (Ti-rich) | $E_{form}$ (O-rich) |
|---|---|---|---|---|
| $O_{Sr}$ | VBM $\rightarrow 0$ | 0.00 | 17.35 | 5.41 |
| | $0 \rightarrow -2$ | 0.63 | 17.35 | 5.41 |
| | $-2 \rightarrow$ CBM | 3.44 | 11.73 | -0.21 |
| $O_{Ti}$ | VBM $\rightarrow 1$ | 0.00 | 24.87 | 9.10 |
| | $1 \rightarrow 0$ | 0.02 | 24.89 | 9.12 |
| | $0 \rightarrow -1$ | 0.72 | 24.89 | 9.12 |
| | $-1 \rightarrow -2$ | 0.85 | 24.76 | 8.99 |
| | $-2 \rightarrow -3$ | 1.16 | 24.14 | 8.38 |
| | $-3 \rightarrow$ CBM | 3.44 | 17.29 | 1.52 |
| $O_{i,I}$ | VBM $\rightarrow 0$ | 0.00 | 7.42 | 1.88 |
| | $0 \rightarrow -1$ | 3.05 | 7.42 | 1.88 |
| | $-1 \rightarrow$ CBM | 3.44 | 7.02 | 1.48 |
| $O_{i,II}$ | VBM $\rightarrow 1$ | 0.00 | 7.07 | 1.52 |
| | $1 \rightarrow -3$ | 2.48 | 9.55 | 4.00 |
| | $-3 \rightarrow$ CBM | 3.44 | 6.66 | 1.12 |
| $Sr_O$ | VBM $\rightarrow 5$ | 0.00 | -5.74 | 6.21 |
| | $5 \rightarrow 4$ | 0.84 | -1.55 | 10.40 |
| | $4 \rightarrow 1$ | 2.90 | 6.68 | 18.63 |
| | $1 \rightarrow$ CBM | 3.44 | 7.23 | 19.17 |
| $Sr_{Ti}$ | VBM $\rightarrow 1$ | 0.00 | 10.02 | 6.19 |
| | $1 \rightarrow 0$ | 0.74 | 10.75 | 6.93 |
| | $0 \rightarrow -1$ | 0.94 | 10.75 | 6.93 |

Continued on next page

TABLE V: **$SrTiO_3$: HSE06**: The transitions levels of native defects in $SrTiO_3$ under Ti-rich and O-rich conditions, calculated using the HSE06 functional. This data corresponds to Figure 6 of the manuscript. (Continued)

| Defect Name | Transition | $E_{Fermi}$ | $E_{form}$ (Ti-rich) | $E_{form}$ (O-rich) |
|---|---|---|---|---|
| | $-1 \rightarrow -2$ | 1.21 | 10.49 | 6.67 |
| | $-2 \rightarrow$ CBM | 3.44 | 6.02 | 2.19 |
| $Sr_{i,I}$ | VBM $\rightarrow 2$ | 0.00 | 0.68 | 7.08 |
| | $2 \rightarrow 1$ | 3.35 | 7.39 | 13.79 |
| | $1 \rightarrow$ CBM | 3.44 | 7.48 | 13.88 |
| $Sr_{i,II}$ | VBM $\rightarrow 2$ | 0.00 | 0.72 | 7.12 |
| | $2 \rightarrow 0$ | 3.39 | 7.49 | 13.90 |
| | $0 \rightarrow$ CBM | 3.44 | 7.49 | 13.90 |
| $Ti_O$ | VBM $\rightarrow 5$ | 0.00 | -8.98 | 6.79 |
| | $5 \rightarrow 3$ | 2.81 | 5.07 | 20.84 |
| | $3 \rightarrow 2$ | 3.26 | 6.43 | 22.20 |
| | $2 \rightarrow 1$ | 3.38 | 6.66 | 22.43 |
| | $1 \rightarrow$ CBM | 3.44 | 6.73 | 22.49 |
| $Ti_{Sr}$ | VBM $\rightarrow 2$ | 0.00 | 0.67 | 4.49 |
| | $2 \rightarrow 1$ | 0.56 | 1.78 | 5.61 |
| | $1 \rightarrow 0$ | 1.23 | 2.46 | 6.28 |
| | $0 \rightarrow$ CBM | 3.44 | 2.46 | 6.28 |
| $Ti_{i,I}$ | VBM $\rightarrow 3$ | 0.00 | -1.12 | 9.11 |
| | $3 \rightarrow 2$ | 1.62 | 3.75 | 13.97 |
| | $2 \rightarrow 1$ | 2.13 | 4.77 | 15.00 |
| | $1 \rightarrow -1$ | 3.05 | 5.69 | 15.91 |
| | $-1 \rightarrow$ CBM | 3.44 | 5.29 | 15.52 |

Continued on next page

TABLE V: **$SrTiO_3$: HSE06**: The transitions levels of native defects in $SrTiO_3$ under Ti-rich and O-rich conditions, calculated using the HSE06 functional. This data corresponds to Figure 6 of the manuscript. (Continued)

| Defect Name | Transition | $E_{\text{Fermi}}$ | $E_{\text{form}}$ (Ti-rich) | $E_{\text{form}}$ (O-rich) |
|---|---|---|---|---|
| $Ti_{i,II}$ | VBM $\rightarrow$ 4 | 0.00 | -6.00 | 4.23 |
| | $4 \rightarrow 3$ | 1.15 | -1.39 | 8.84 |
| | $3 \rightarrow 2$ | 3.06 | 4.32 | 14.55 |
| | $2 \rightarrow 0$ | 3.34 | 4.90 | 15.12 |
| | $0 \rightarrow$ CBM | 3.44 | 4.90 | 15.12 |
| $v_O$ | VBM $\rightarrow$ 2 | 0.00 | -6.53 | -0.98 |
| | $2 \rightarrow 1$ | 3.33 | 0.13 | 5.67 |
| | $1 \rightarrow$ CBM | 3.44 | 0.24 | 5.79 |
| $v_{Sr}$ | VBM $\rightarrow$ 1 | 0.00 | 9.44 | 3.04 |
| | $1 \rightarrow 0$ | 0.07 | 9.51 | 3.10 |
| | $0 \rightarrow -1$ | 0.28 | 9.51 | 3.10 |
| | $-1 \rightarrow -2$ | 0.40 | 9.39 | 2.99 |
| | $-2 \rightarrow$ CBM | 3.44 | 3.30 | -3.11 |
| $v_{Ti}$ | VBM $\rightarrow$ 1 | 0.00 | 16.20 | 5.98 |
| | $1 \rightarrow -1$ | 0.73 | 16.93 | 6.71 |
| | $-1 \rightarrow -4$ | 1.03 | 16.64 | 6.41 |
| | $-4 \rightarrow$ CBM | 3.44 | 6.97 | -3.26 |
